# Supplementary material for: Physical and chemical properties of Wolf-Rayet planetary nebulae
Source: arXiv:2106.10762 source file (2021-08-26)
Supplement: Supplementary file 1 [file extinction.tex]

\noalign{\smallskip}
\hline
\noalign{\smallskip}
\multicolumn{5}{c}{PB 6          (PNG278.8+04.9) }\\
\noalign{\smallskip}
\hline
\noalign{\smallskip}
H$^{+}$    &H~{\sc i}        $\lambda$6562.77  & B3   &    1 & $ 5.432_{-0.312}^{+ 0.361} \times 10^{  -1}$ \\
\noalign{\smallskip}
\hline
\noalign{\smallskip}
H$^{+}$    &Total             &  &  & $ 5.432_{-0.312}^{+ 0.361} \times 10^{  -1}$ \\
\noalign{\smallskip}
\hline
\noalign{\smallskip}
\multicolumn{5}{c}{M 3-30        (PNG017.9-04.8) }\\
\noalign{\smallskip}
\hline
\noalign{\smallskip}
H$^{+}$    &H~{\sc i}        $\lambda$6562.77  & B3   &    1 & $ 1.005_{-0.013}^{+ 0.013} \times 10^{   0}$ \\
\noalign{\smallskip}
\hline
\noalign{\smallskip}
H$^{+}$    &Total             &  &  & $ 1.005_{-0.013}^{+ 0.013} \times 10^{   0}$ \\
\noalign{\smallskip}
\hline
\noalign{\smallskip}
\multicolumn{5}{c}{Hb 4 (shell)  (PNG003.1+02.9) }\\
\noalign{\smallskip}
\hline
\noalign{\smallskip}
H$^{+}$    &H~{\sc i}        $\lambda$6562.77  & B3   &    1 & $ 1.851_{-0.009}^{+ 0.008} \times 10^{   0}$ \\
\noalign{\smallskip}
\hline
\noalign{\smallskip}
H$^{+}$    &Total             &  &  & $ 1.851_{-0.009}^{+ 0.008} \times 10^{   0}$ \\
\noalign{\smallskip}
\hline
\noalign{\smallskip}
\multicolumn{5}{c}{Hb 4 (N-knot) (PNG003.1+02.9) }\\
\noalign{\smallskip}
\hline
\noalign{\smallskip}
H$^{+}$    &H~{\sc i}        $\lambda$6562.77  & B3   &    1 & $ 2.089_{-0.033}^{+ 0.029} \times 10^{   0}$ \\
\noalign{\smallskip}
\hline
\noalign{\smallskip}
H$^{+}$    &Total             &  &  & $ 2.089_{-0.033}^{+ 0.029} \times 10^{   0}$ \\
\noalign{\smallskip}
\hline
\noalign{\smallskip}
\multicolumn{5}{c}{Hb 4 (S-knot) (PNG003.1+02.9) }\\
\noalign{\smallskip}
\hline
\noalign{\smallskip}
H$^{+}$    &H~{\sc i}        $\lambda$6562.77  & B3   &    1 & $ 1.908_{-0.057}^{+ 0.045} \times 10^{   0}$ \\
\noalign{\smallskip}
\hline
\noalign{\smallskip}
H$^{+}$    &Total             &  &  & $ 1.908_{-0.057}^{+ 0.045} \times 10^{   0}$ \\
\noalign{\smallskip}
\hline
\noalign{\smallskip}
\multicolumn{5}{c}{IC 1297       (PNG358.3-21.6) }\\
\noalign{\smallskip}
\hline
\noalign{\smallskip}
H$^{+}$    &H~{\sc i}        $\lambda$6562.77  & B3   &    1 & $ 2.209_{-0.127}^{+ 0.147} \times 10^{  -1}$ \\
\noalign{\smallskip}
\hline
\noalign{\smallskip}
H$^{+}$    &Total             &  &  & $ 2.209_{-0.127}^{+ 0.147} \times 10^{  -1}$ \\
\noalign{\smallskip}
\hline
\noalign{\smallskip}
\multicolumn{5}{c}{Th 2-A        (PNG306.4-00.6) }\\
\noalign{\smallskip}
\hline
\noalign{\smallskip}
H$^{+}$    &H~{\sc i}        $\lambda$6562.77  & B3   &    1 & $ 1.079_{-0.021}^{+ 0.022} \times 10^{   0}$ \\
\noalign{\smallskip}
\hline
\noalign{\smallskip}
H$^{+}$    &Total             &  &  & $ 1.079_{-0.021}^{+ 0.022} \times 10^{   0}$ \\
\noalign{\smallskip}
\hline
\noalign{\smallskip}
\multicolumn{5}{c}{Pe 1-1        (PNG285.4+01.5) }\\
\noalign{\smallskip}
\hline
\noalign{\smallskip}
H$^{+}$    &H~{\sc i}        $\lambda$6562.77  & B3   &    1 & $ 1.943_{-0.007}^{+ 0.005} \times 10^{   0}$ \\
\noalign{\smallskip}
\hline
\noalign{\smallskip}
H$^{+}$    &Total             &  &  & $ 1.943_{-0.007}^{+ 0.005} \times 10^{   0}$ \\
\noalign{\smallskip}
\hline
\noalign{\smallskip}
\multicolumn{5}{c}{M 1-32        (PNG011.9+04.2) }\\
\noalign{\smallskip}
\hline
\noalign{\smallskip}
H$^{+}$    &H~{\sc i}        $\lambda$6562.77  & B3   &    1 & $ 1.347_{-0.028}^{+ 0.024} \times 10^{   0}$ \\
\noalign{\smallskip}
\hline
\noalign{\smallskip}
H$^{+}$    &Total             &  &  & $ 1.347_{-0.028}^{+ 0.024} \times 10^{   0}$ \\
\noalign{\smallskip}
\hline
\noalign{\smallskip}
\multicolumn{5}{c}{M 3-15        (PNG006.8+04.1) }\\
\noalign{\smallskip}
\hline
\noalign{\smallskip}
H$^{+}$    &H~{\sc i}        $\lambda$6562.77  & B3   &    1 & $ 2.251_{-0.011}^{+ 0.010} \times 10^{   0}$ \\
\noalign{\smallskip}
\hline
\noalign{\smallskip}
H$^{+}$    &Total             &  &  & $ 2.251_{-0.011}^{+ 0.010} \times 10^{   0}$ \\
\noalign{\smallskip}
\hline
\noalign{\smallskip}
\multicolumn{5}{c}{M 1-25        (PNG004.9+04.9) }\\
\noalign{\smallskip}
\hline
\noalign{\smallskip}
H$^{+}$    &H~{\sc i}        $\lambda$6562.77  & B3   &    1 & $ 1.596_{-0.004}^{+ 0.005} \times 10^{   0}$ \\
\noalign{\smallskip}
\hline
\noalign{\smallskip}
H$^{+}$    &Total             &  &  & $ 1.596_{-0.004}^{+ 0.005} \times 10^{   0}$ \\
\noalign{\smallskip}
\hline
\noalign{\smallskip}
\multicolumn{5}{c}{Hen 2-142     (PNG327.1-02.2) }\\
\noalign{\smallskip}
\hline
\noalign{\smallskip}
H$^{+}$    &H~{\sc i}        $\lambda$6562.77  & B3   &    1 & $ 1.554_{-0.087}^{+ 0.091} \times 10^{   0}$ \\
\noalign{\smallskip}
\hline
\noalign{\smallskip}
H$^{+}$    &Total             &  &  & $ 1.554_{-0.087}^{+ 0.091} \times 10^{   0}$ \\
\noalign{\smallskip}
\hline
\noalign{\smallskip}
\multicolumn{5}{c}{Hen 3-1333    (PNG332.9-09.9) }\\
\noalign{\smallskip}
\hline
\noalign{\smallskip}
H$^{+}$    &H~{\sc i}        $\lambda$6562.77  & B3   &    1 & $ 1.064_{-0.021}^{+ 0.020} \times 10^{   0}$ \\
\noalign{\smallskip}
\hline
\noalign{\smallskip}
H$^{+}$    &Total             &  &  & $ 9.598_{-0.231}^{+ 0.247} \times 10^{  -1}$ \\
\noalign{\smallskip}
\hline
\noalign{\smallskip}
\multicolumn{5}{c}{Hen 2-113     (PNG321.0+03.9) }\\
\noalign{\smallskip}
\hline
\noalign{\smallskip}
H$^{+}$    &H~{\sc i}        $\lambda$6562.77  & B3   &    1 & $ 1.335_{-0.025}^{+ 0.028} \times 10^{   0}$ \\
\noalign{\smallskip}
\hline
\noalign{\smallskip}
H$^{+}$    &Total             &  &  & $ 1.335_{-0.025}^{+ 0.028} \times 10^{   0}$ \\
\noalign{\smallskip}
\hline
\noalign{\smallskip}
\multicolumn{5}{c}{K 2-16        (PNG352.9+11.4) }\\
\noalign{\smallskip}
\hline
\noalign{\smallskip}
H$^{+}$    &H~{\sc i}        $\lambda$6562.77  & B3   &    1 & $ 4.992_{-0.399}^{+ 0.428} \times 10^{  -1}$ \\
\noalign{\smallskip}
\hline
\noalign{\smallskip}
H$^{+}$    &Total             &  &  & $ 4.992_{-0.399}^{+ 0.428} \times 10^{  -1}$ \\
\noalign{\smallskip}
\hline
\noalign{\smallskip}
\multicolumn{5}{c}{NGC 6578      (PNG010.8-01.8) }\\
\noalign{\smallskip}
\hline
\noalign{\smallskip}
H$^{+}$    &H~{\sc i}        $\lambda$6562.77  & B3   &    1 & $ 1.510_{-0.009}^{+ 0.010} \times 10^{   0}$ \\
\noalign{\smallskip}
\hline
\noalign{\smallskip}
H$^{+}$    &Total             &  &  & $ 1.510_{-0.009}^{+ 0.010} \times 10^{   0}$ \\
\noalign{\smallskip}
\hline
\noalign{\smallskip}
\multicolumn{5}{c}{M 2-42        (PNG008.2-04.8) }\\
\noalign{\smallskip}
\hline
\noalign{\smallskip}
H$^{+}$    &H~{\sc i}        $\lambda$6562.77  & B3   &    1 & $ 9.790_{-0.279}^{+ 0.313} \times 10^{  -1}$ \\
\noalign{\smallskip}
\hline
\noalign{\smallskip}
H$^{+}$    &Total             &  &  & $ 9.790_{-0.279}^{+ 0.313} \times 10^{  -1}$ \\
\noalign{\smallskip}
\hline
\noalign{\smallskip}
\multicolumn{5}{c}{NGC 6567      (PNG011.7-00.6) }\\
\noalign{\smallskip}
\hline
\noalign{\smallskip}
H$^{+}$    &H~{\sc i}        $\lambda$6562.77  & B3   &    1 & $ 7.696_{-0.062}^{+ 0.079} \times 10^{  -1}$ \\
\noalign{\smallskip}
\hline
\noalign{\smallskip}
H$^{+}$    &Total             &  &  & $ 7.696_{-0.062}^{+ 0.079} \times 10^{  -1}$ \\
\noalign{\smallskip}
\hline
\noalign{\smallskip}
\multicolumn{5}{c}{NGC 6629      (PNG009.4-05.0) }\\
\noalign{\smallskip}
\hline
\noalign{\smallskip}
H$^{+}$    &H~{\sc i}        $\lambda$6562.77  & B3   &    1 & $ 9.745_{-0.089}^{+ 0.082} \times 10^{  -1}$ \\
\noalign{\smallskip}
\hline
\noalign{\smallskip}
H$^{+}$    &Total             &  &  & $ 9.745_{-0.089}^{+ 0.082} \times 10^{  -1}$ \\
\noalign{\smallskip}
\hline
\noalign{\smallskip}
\multicolumn{5}{c}{Sa 3-107      (PNG358.0-04.6) }\\
\noalign{\smallskip}
\hline
\noalign{\smallskip}
H$^{+}$    &H~{\sc i}        $\lambda$6562.77  & B3   &    1 & $ 1.616_{-0.010}^{+ 0.009} \times 10^{   0}$ \\
\noalign{\smallskip}
\hline
\noalign{\smallskip}
H$^{+}$    &Total             &  &  & $ 1.616_{-0.010}^{+ 0.009} \times 10^{   0}$ \\
