# Supplementary material for: Physical and chemical properties of Wolf-Rayet planetary nebulae
Source: arXiv:2106.10762 source file (2021-08-26)
Supplement: Supplementary file 2 [file abundance_adf.tex]

\noalign{\smallskip}
\hline
\noalign{\smallskip}
\multicolumn{4}{c}{PB 6          (PNG278.8+04.9) }\\
\noalign{\smallskip}
\hline
\noalign{\smallskip}
{\it adf}(N$^{2+}$)       & ORL/CEL &          & $      26.782_{      -2.402}^{+       2.406}$ \\
\noalign{\smallskip}
{\it adf}(N)              & ORL/CEL & KB94     & $      11.292_{      -1.345}^{+       1.123}$ \\
\noalign{\smallskip}
{\it adf}(N)              & ORL/CEL & DMS14    & $      12.997_{     -12.997}^{+      48.697}$ \\
\noalign{\smallskip}
\noalign{\medskip}
{\it adf}(O$^{2+}$)       & ORL/CEL &          & $       4.295_{      -1.245}^{+       1.097}$ \\
\noalign{\smallskip}
{\it adf}(O)              & ORL/CEL & KB94     & $       4.295_{      -1.470}^{+       1.452}$ \\
\noalign{\smallskip}
{\it adf}(O)              & ORL/CEL & DMS14    & $       3.923_{      -2.141}^{+       3.117}$ \\
\noalign{\smallskip}
\hline
\noalign{\smallskip}
\multicolumn{4}{c}{M 3-30        (PNG017.9-04.8) }\\
\noalign{\smallskip}
\hline
\noalign{\smallskip}
{\it adf}(N$^{2+}$)       & ORL/CEL &          & $      22.439_{      -2.274}^{+       2.369}$ \\
\noalign{\smallskip}
{\it adf}(N)              & ORL/CEL & KB94     & $      22.439_{      -2.842}^{+       2.776}$ \\
\noalign{\smallskip}
{\it adf}(N)              & ORL/CEL & DMS14    & $      28.173_{     -28.173}^{+   13975.388}$ \\
\noalign{\smallskip}
\noalign{\medskip}
{\it adf}(O$^{2+}$)       & ORL/CEL &          & $      14.995_{      -1.576}^{+       1.617}$ \\
\noalign{\smallskip}
{\it adf}(O)              & ORL/CEL & KB94     & $      14.995_{      -1.891}^{+       1.970}$ \\
\noalign{\smallskip}
{\it adf}(O)              & ORL/CEL & DMS14    & $      15.129_{      -4.314}^{+       8.191}$ \\
\noalign{\smallskip}
\hline
\noalign{\smallskip}
\multicolumn{4}{c}{Hb 4 (shell)  (PNG003.1+02.9) }\\
\noalign{\smallskip}
\hline
\noalign{\smallskip}
{\it adf}(N$^{2+}$)       & ORL/CEL &          & $       3.165_{      -0.488}^{+       0.480}$ \\
\noalign{\smallskip}
{\it adf}(N)              & ORL/CEL & KB94     & $       3.165_{      -0.610}^{+       0.604}$ \\
\noalign{\smallskip}
{\it adf}(N)              & ORL/CEL & DMS14    & $       3.178_{      -3.178}^{+     147.533}$ \\
\noalign{\smallskip}
\noalign{\medskip}
{\it adf}(O$^{2+}$)       & ORL/CEL &          & $       9.795_{      -1.265}^{+       1.488}$ \\
\noalign{\smallskip}
{\it adf}(O)              & ORL/CEL & KB94     & $       9.795_{      -1.565}^{+       1.912}$ \\
\noalign{\smallskip}
{\it adf}(O)              & ORL/CEL & DMS14    & $       9.899_{      -1.717}^{+       2.248}$ \\
\noalign{\smallskip}
\hline
\noalign{\smallskip}
\multicolumn{4}{c}{IC 1297       (PNG358.3-21.6) }\\
\noalign{\smallskip}
\hline
\noalign{\smallskip}
{\it adf}(N$^{2+}$)       & ORL/CEL &          & $       2.838_{      -0.524}^{+       0.691}$ \\
\noalign{\smallskip}
{\it adf}(N)              & ORL/CEL & KB94     & $       8.080_{      -0.726}^{+       0.971}$ \\
\noalign{\smallskip}
{\it adf}(N)              & ORL/CEL & DMS14    & $       9.421_{      -9.421}^{+      21.019}$ \\
\noalign{\smallskip}
\noalign{\medskip}
{\it adf}(O$^{2+}$)       & ORL/CEL &          & $       2.122_{      -0.248}^{+       0.256}$ \\
\noalign{\smallskip}
{\it adf}(O)              & ORL/CEL & KB94     & $       2.122_{      -0.324}^{+       0.350}$ \\
\noalign{\smallskip}
{\it adf}(O)              & ORL/CEL & DMS14    & $       2.164_{      -0.510}^{+       0.684}$ \\
\noalign{\smallskip}
\hline
\noalign{\smallskip}
\multicolumn{4}{c}{Th 2-A        (PNG306.4-00.6) }\\
\noalign{\smallskip}
\hline
\noalign{\smallskip}
{\it adf}(N$^{2+}$)       & ORL/CEL &          & $      46.116_{      -5.566}^{+       7.125}$ \\
\noalign{\smallskip}
{\it adf}(N)              & ORL/CEL & KB94     & $      29.196_{      -5.241}^{+       7.162}$ \\
\noalign{\smallskip}
{\it adf}(N)              & ORL/CEL & DMS14    & $      33.472_{     -33.472}^{+     148.020}$ \\
\noalign{\smallskip}
\noalign{\medskip}
{\it adf}(O$^{2+}$)       & ORL/CEL &          & $      24.528_{      -3.331}^{+       4.277}$ \\
\noalign{\smallskip}
{\it adf}(O)              & ORL/CEL & KB94     & $      24.528_{      -4.209}^{+       5.868}$ \\
\noalign{\smallskip}
{\it adf}(O)              & ORL/CEL & DMS14    & $      24.913_{      -6.856}^{+      14.877}$ \\
\noalign{\smallskip}
\hline
\noalign{\smallskip}
\multicolumn{4}{c}{Pe 1-1        (PNG285.4+01.5) }\\
\noalign{\smallskip}
\hline
\noalign{\smallskip}
{\it adf}(N$^{2+}$)       & ORL/CEL &          & $      16.976_{      -4.514}^{+       5.356}$ \\
\noalign{\smallskip}
{\it adf}(N)              & ORL/CEL & KB94     & $      16.976_{      -7.107}^{+       8.224}$ \\
\noalign{\smallskip}
{\it adf}(N)              & ORL/CEL & DMS14    & $       5.572_{      -5.572}^{+      38.969}$ \\
\noalign{\smallskip}
\noalign{\medskip}
{\it adf}(O$^{2+}$)       & ORL/CEL &          & $       6.292_{      -1.678}^{+       1.321}$ \\
\noalign{\smallskip}
{\it adf}(O)              & ORL/CEL & KB94     & $       6.292_{      -2.370}^{+       1.947}$ \\
\noalign{\smallskip}
{\it adf}(O)              & ORL/CEL & DMS14    & $       6.292_{      -2.357}^{+       1.963}$ \\
\noalign{\smallskip}
\hline
\noalign{\smallskip}
\multicolumn{4}{c}{M 1-32        (PNG011.9+04.2) }\\
\noalign{\smallskip}
\hline
\noalign{\smallskip}
{\it adf}(N$^{2+}$)       & ORL/CEL &          & $       8.947_{      -1.623}^{+       1.703}$ \\
\noalign{\smallskip}
{\it adf}(N)              & ORL/CEL & KB94     & $       8.947_{      -2.170}^{+       2.574}$ \\
\noalign{\smallskip}
{\it adf}(N)              & ORL/CEL & DMS14    & $       3.793_{      -2.744}^{+       4.043}$ \\
\noalign{\smallskip}
\noalign{\medskip}
{\it adf}(O$^{2+}$)       & ORL/CEL &          & $      27.687_{      -9.691}^{+      10.381}$ \\
\noalign{\smallskip}
{\it adf}(O)              & ORL/CEL & KB94     & $      27.687_{     -12.226}^{+      14.263}$ \\
\noalign{\smallskip}
{\it adf}(O)              & ORL/CEL & DMS14    & $      27.687_{     -12.631}^{+      14.103}$ \\
\noalign{\smallskip}
\hline
\noalign{\smallskip}
\multicolumn{4}{c}{M 3-15        (PNG006.8+04.1) }\\
\noalign{\smallskip}
\hline
\noalign{\smallskip}
{\it adf}(N$^{2+}$)       & ORL/CEL &          & $      12.433_{      -3.532}^{+       3.357}$ \\
\noalign{\smallskip}
{\it adf}(N)              & ORL/CEL & KB94     & $      12.433_{      -4.346}^{+       4.141}$ \\
\noalign{\smallskip}
{\it adf}(N)              & ORL/CEL & DMS14    & $       3.332_{      -3.332}^{+       5.643}$ \\
\noalign{\smallskip}
\hline
\noalign{\smallskip}
\multicolumn{4}{c}{M 1-25        (PNG004.9+04.9) }\\
\noalign{\smallskip}
\hline
\noalign{\smallskip}
{\it adf}(N$^{2+}$)       & ORL/CEL &          & $      16.687_{      -2.541}^{+       2.713}$ \\
\noalign{\smallskip}
{\it adf}(N)              & ORL/CEL & KB94     & $      16.687_{      -3.364}^{+       3.022}$ \\
\noalign{\smallskip}
{\it adf}(N)              & ORL/CEL & DMS14    & $       6.990_{      -4.578}^{+      19.050}$ \\
\noalign{\smallskip}
\noalign{\medskip}
{\it adf}(O$^{2+}$)       & ORL/CEL &          & $      11.048_{      -1.831}^{+       1.909}$ \\
\noalign{\smallskip}
{\it adf}(O)              & ORL/CEL & KB94     & $      11.048_{      -2.276}^{+       2.270}$ \\
\noalign{\smallskip}
{\it adf}(O)              & ORL/CEL & DMS14    & $      11.048_{      -2.322}^{+       2.188}$ \\
\noalign{\smallskip}
\hline
\noalign{\smallskip}
\multicolumn{4}{c}{NGC 6578      (PNG010.8-01.8) }\\
\noalign{\smallskip}
\hline
\noalign{\smallskip}
{\it adf}(N$^{2+}$)       & ORL/CEL &          & $      11.370_{      -2.764}^{+       2.761}$ \\
\noalign{\smallskip}
{\it adf}(N)              & ORL/CEL & KB94     & $      13.485_{      -5.171}^{+       4.437}$ \\
\noalign{\smallskip}
{\it adf}(N)              & ORL/CEL & DMS14    & $       8.137_{      -8.137}^{+      81.933}$ \\
\noalign{\smallskip}
\noalign{\medskip}
{\it adf}(O$^{2+}$)       & ORL/CEL &          & $       6.284_{      -0.975}^{+       0.980}$ \\
\noalign{\smallskip}
{\it adf}(O)              & ORL/CEL & KB94     & $       6.284_{      -1.234}^{+       1.354}$ \\
\noalign{\smallskip}
{\it adf}(O)              & ORL/CEL & DMS14    & $       6.287_{      -1.252}^{+       1.400}$ \\
\noalign{\smallskip}
\hline
\noalign{\smallskip}
\multicolumn{4}{c}{M 2-42        (PNG008.2-04.8) }\\
\noalign{\smallskip}
\hline
\noalign{\smallskip}
{\it adf}(N$^{2+}$)       & ORL/CEL &          & $      24.556_{      -1.702}^{+       2.012}$ \\
\noalign{\smallskip}
{\it adf}(N)              & ORL/CEL & KB94     & $      26.225_{      -2.038}^{+       2.870}$ \\
\noalign{\smallskip}
{\it adf}(N)              & ORL/CEL & DMS14    & $      15.432_{     -15.432}^{+     169.433}$ \\
\noalign{\smallskip}
\noalign{\medskip}
{\it adf}(O$^{2+}$)       & ORL/CEL &          & $       3.603_{      -0.722}^{+       0.509}$ \\
\noalign{\smallskip}
{\it adf}(O)              & ORL/CEL & KB94     & $       3.603_{      -0.779}^{+       0.607}$ \\
\noalign{\smallskip}
{\it adf}(O)              & ORL/CEL & DMS14    & $       3.605_{      -0.768}^{+       0.639}$ \\
\noalign{\smallskip}
\hline
\noalign{\smallskip}
\multicolumn{4}{c}{NGC 6567      (PNG011.7-00.6) }\\
\noalign{\smallskip}
\hline
\noalign{\smallskip}
{\it adf}(N$^{2+}$)       & ORL/CEL &          & $      61.727_{     -10.925}^{+      11.067}$ \\
\noalign{\smallskip}
{\it adf}(N)              & ORL/CEL & KB94     & $      61.727_{     -15.105}^{+      14.245}$ \\
\noalign{\smallskip}
{\it adf}(N)              & ORL/CEL & DMS14    & $      40.881_{     -40.881}^{+     310.249}$ \\
\noalign{\smallskip}
\noalign{\medskip}
{\it adf}(O$^{2+}$)       & ORL/CEL &          & $      28.163_{      -5.486}^{+       5.085}$ \\
\noalign{\smallskip}
{\it adf}(O)              & ORL/CEL & KB94     & $      28.163_{      -7.155}^{+       6.629}$ \\
\noalign{\smallskip}
{\it adf}(O)              & ORL/CEL & DMS14    & $      28.184_{      -7.277}^{+       6.628}$ \\
\noalign{\smallskip}
\hline
\noalign{\smallskip}
\multicolumn{4}{c}{NGC 6629      (PNG009.4-05.0) }\\
\noalign{\smallskip}
\hline
\noalign{\smallskip}
{\it adf}(O$^{2+}$)       & ORL/CEL &          & $       2.267_{      -0.598}^{+       0.444}$ \\
\noalign{\smallskip}
{\it adf}(O)              & ORL/CEL & KB94     & $       2.267_{      -0.725}^{+       0.643}$ \\
\noalign{\smallskip}
{\it adf}(O)              & ORL/CEL & DMS14    & $       2.267_{      -0.717}^{+       0.673}$ \\
\noalign{\smallskip}
\hline
\noalign{\smallskip}
\multicolumn{4}{c}{Sa 3-107      (PNG358.0-04.6) }\\
\noalign{\smallskip}
\hline
\noalign{\smallskip}
{\it adf}(N$^{2+}$)       & ORL/CEL &          & $      25.940_{     -25.940}^{+     689.698}$ \\
\noalign{\smallskip}
{\it adf}(N)              & ORL/CEL & KB94     & $      29.715_{     -29.715}^{+     690.154}$ \\
\noalign{\smallskip}
{\it adf}(N)              & ORL/CEL & DMS14    & $      21.063_{     -21.063}^{+    2745.244}$ \\
